# Supplementary material for: Unsupervised Novel View Synthesis from a Single Image
Source: arXiv:2102.03285 source file (2021-12-15)
Supplement: Supplementary file 1 [file fitting_strategies.tex]

 % \cite{creswellTNNL2019}, 2) \cite{zhuECCV2016}, 3) \cite{zhuECCV2016} applied with our Stage 2 network already finetuned on the whole dataset but keeping $D$ frozen, and finally 4) our finetuning.
 \begin{figure*}
	\setlength{\tabcolsep}{1pt}
	\centering
	\setlength{\fboxrule}{2pt} 
	\setlength{\fboxsep}{0pt} 
	\scalebox{0.9}{
	\begin{tabular}{cc|cccc|c|cccc}
	&Input. & \multicolumn{4}{|c|}{$\theta$ Interpolation} & Input. & \multicolumn{4}{c}{$\theta$ Interpolation}\\
	\rotatebox{90}{\hspace{0.7cm}\cite{creswellTNNL2019}} &
    \includegraphics[width=0.10\textwidth]{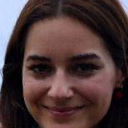} & \includegraphics[width=0.10\textwidth]{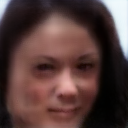} & \includegraphics[width=0.10\textwidth]{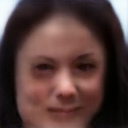} & \includegraphics[width=0.10\textwidth]{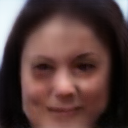} & \includegraphics[width=0.10\textwidth]{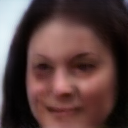} &
     \includegraphics[width=0.10\textwidth]{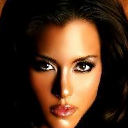} & \includegraphics[width=0.10\textwidth]{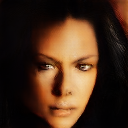} & \includegraphics[width=0.10\textwidth]{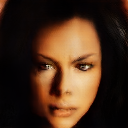} & \includegraphics[width=0.10\textwidth]{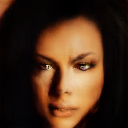} & \includegraphics[width=0.10\textwidth]{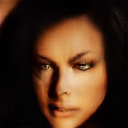} \\
     \rotatebox{90}{\hspace{0.6cm}\cite{zhuECCV2016}} &
     \includegraphics[width=0.10\textwidth]{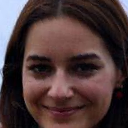} & \includegraphics[width=0.10\textwidth]{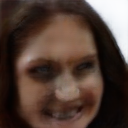} & \includegraphics[width=0.10\textwidth]{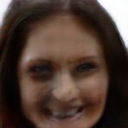} & \includegraphics[width=0.10\textwidth]{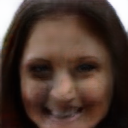} & \includegraphics[width=0.10\textwidth]{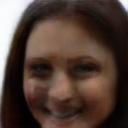} &
      \includegraphics[width=0.10\textwidth]{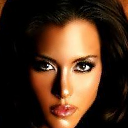} & \includegraphics[width=0.10\textwidth]{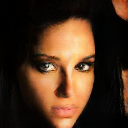} & \includegraphics[width=0.10\textwidth]{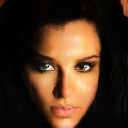} & \includegraphics[width=0.10\textwidth]{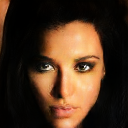} & \includegraphics[width=0.10\textwidth]{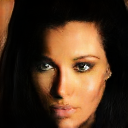} \\
      \rotatebox{90}{\hspace{0.6cm}\cite{zhuECCV2016}}\rotatebox{90}{\vspace{2mm}w/ Stage 2} &
     \includegraphics[width=0.10\textwidth]{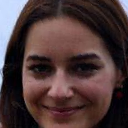} & \includegraphics[width=0.10\textwidth]{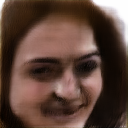} & \includegraphics[width=0.10\textwidth]{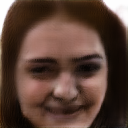} & \includegraphics[width=0.10\textwidth]{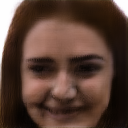} & \includegraphics[width=0.10\textwidth]{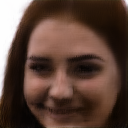} &
      \includegraphics[width=0.10\textwidth]{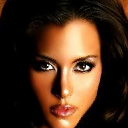} & \includegraphics[width=0.10\textwidth]{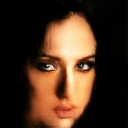} & \includegraphics[width=0.10\textwidth]{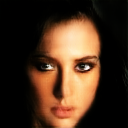} & \includegraphics[width=0.10\textwidth]{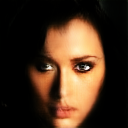} & \includegraphics[width=0.10\textwidth]{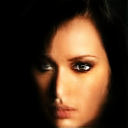} \\
     
     \vspace{0.2cm}
     \rotatebox{90}{\hspace{0.5cm}Ours} &
     \includegraphics[width=0.10\textwidth]{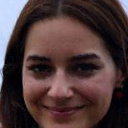} & \includegraphics[width=0.10\textwidth]{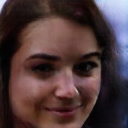} & \includegraphics[width=0.10\textwidth]{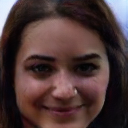} & \includegraphics[width=0.10\textwidth]{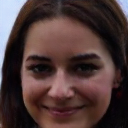} & \includegraphics[width=0.10\textwidth]{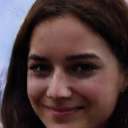} &
     \includegraphics[width=0.10\textwidth]{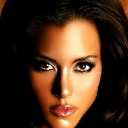} & \includegraphics[width=0.10\textwidth]{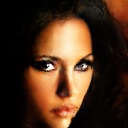} & \includegraphics[width=0.10\textwidth]{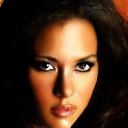} & \includegraphics[width=0.10\textwidth]{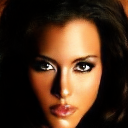} & \includegraphics[width=0.10\textwidth]{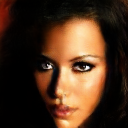} \\
    
     \rotatebox{90}{\hspace{0.7cm}\cite{creswellTNNL2019}} &
     \includegraphics[width=0.10\textwidth]{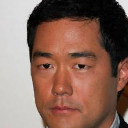} & \includegraphics[width=0.10\textwidth]{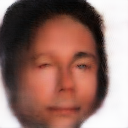} & \includegraphics[width=0.10\textwidth]{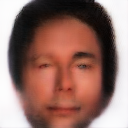} & \includegraphics[width=0.10\textwidth]{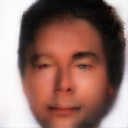} & \includegraphics[width=0.10\textwidth]{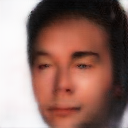} &
      \includegraphics[width=0.10\textwidth]{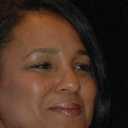} & \includegraphics[width=0.10\textwidth]{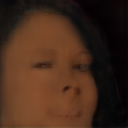} & \includegraphics[width=0.10\textwidth]{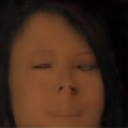} & \includegraphics[width=0.10\textwidth]{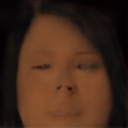} & \includegraphics[width=0.10\textwidth]{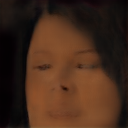} \\
     \rotatebox{90}{\hspace{0.6cm}\cite{zhuECCV2016}} &
     \includegraphics[width=0.10\textwidth]{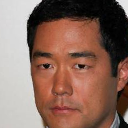} & \includegraphics[width=0.10\textwidth]{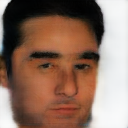} & \includegraphics[width=0.10\textwidth]{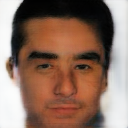} & \includegraphics[width=0.10\textwidth]{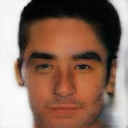} & \includegraphics[width=0.10\textwidth]{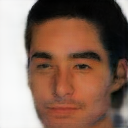} &
     \includegraphics[width=0.10\textwidth]{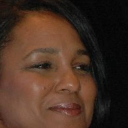} & \includegraphics[width=0.10\textwidth]{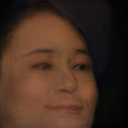} & \includegraphics[width=0.10\textwidth]{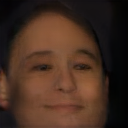} & \includegraphics[width=0.10\textwidth]{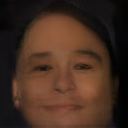} & \includegraphics[width=0.10\textwidth]{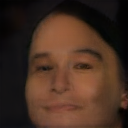} \\
     \rotatebox{90}{\hspace{0.6cm}\cite{zhuECCV2016}}\rotatebox{90}{\vspace{2mm}w/ Stage 2} &
     \includegraphics[width=0.10\textwidth]{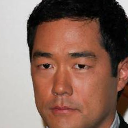} & \includegraphics[width=0.10\textwidth]{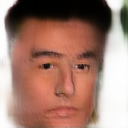} & \includegraphics[width=0.10\textwidth]{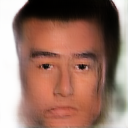} & \includegraphics[width=0.10\textwidth]{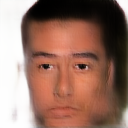} & \includegraphics[width=0.10\textwidth]{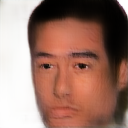} &
     \includegraphics[width=0.10\textwidth]{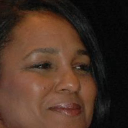} & \includegraphics[width=0.10\textwidth]{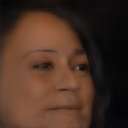} & \includegraphics[width=0.10\textwidth]{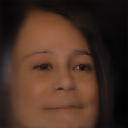} & \includegraphics[width=0.10\textwidth]{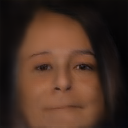} & \includegraphics[width=0.10\textwidth]{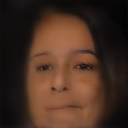} \\
     \rotatebox{90}{\hspace{0.5cm}Ours} &
     \includegraphics[width=0.10\textwidth]{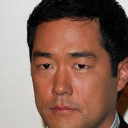} & \includegraphics[width=0.10\textwidth]{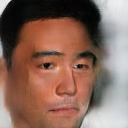} & \includegraphics[width=0.10\textwidth]{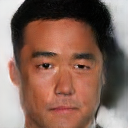} & \includegraphics[width=0.10\textwidth]{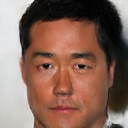} & \includegraphics[width=0.10\textwidth]{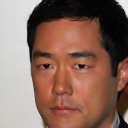} &
     \includegraphics[width=0.10\textwidth]{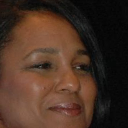} & \includegraphics[width=0.10\textwidth]{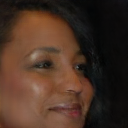} & \includegraphics[width=0.10\textwidth]{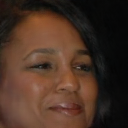} & \includegraphics[width=0.10\textwidth]{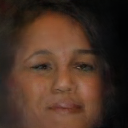} & \includegraphics[width=0.10\textwidth]{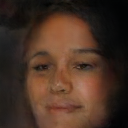} \\
	\end{tabular}}
	%\caption{Each 5 by 4 blocks shows different strategies to fit the same input image from the CelebA test set. From the first to the fourth row of each block: \textit{Fitting} \cite{creswellTNNL2019} HoloGAN, \textit{Fitting} \cite{creswellTNNL2019} a Stage 1 Network, \textit{Fitting} \cite{creswellTNNL2019} a Stage 2 Network, Our Fine-Tuning. For \textit{Fitting} Stage 1, \textit{Fitting} Stage 2 and \textit{Fine-tuning} we initialize $z$ and $\theta$ from the output of the encoder $E$.}
	\caption{Each $4\times 5$ block shows different strategies to fit the same input image from the CelebA test set. From first to fourth row of each block: \textit{Fitting} \cite{creswellTNNL2019} HoloGAN, \textit{Fitting} \cite{creswellTNNL2019} a Stage 1 Network, \textit{Fitting} \cite{creswellTNNL2019} a Stage 2 Network, Our Fine-Tuning. For the last three rows we initialize $z$ and $\theta$ from the output of the encoder $E$.}
	\label{fig:fitting_strategies}
\end{figure*}
