# Supplementary material for: Unsupervised Novel View Synthesis from a Single Image
Source: arXiv:2102.03285 source file (2021-12-15)
Supplement: Supplementary file 2 [file comparison_cfgnet.tex]

\begin{figure*}
	\setlength{\tabcolsep}{1pt}
	\centering
	\setlength{\fboxrule}{2pt} 
	\setlength{\fboxsep}{0pt} 
	\scalebox{0.9}{
	\begin{tabular}{cc|cccccccc}
	& Input. & \multicolumn{8}{|c|}{$\theta$ Interpolation} \\
    \rotatebox{90}{\hspace{0.5cm} Ours} &
	\includegraphics[width=0.115\textwidth]{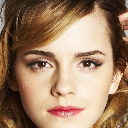} & \includegraphics[width=0.115\textwidth]{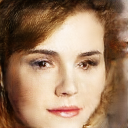} & \includegraphics[width=0.115\textwidth]{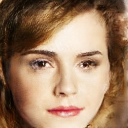} & \includegraphics[width=0.115\textwidth]{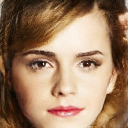} & \includegraphics[width=0.115\textwidth]{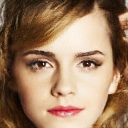} & \includegraphics[width=0.115\textwidth]{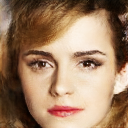} & \includegraphics[width=0.115\textwidth]{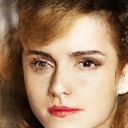} & \includegraphics[width=0.115\textwidth]{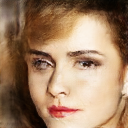} & \includegraphics[width=0.115\textwidth]{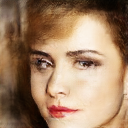} \\
     \rotatebox{90}{\hspace{0.2cm} ConfigNet} &
    \includegraphics[width=0.115\textwidth]{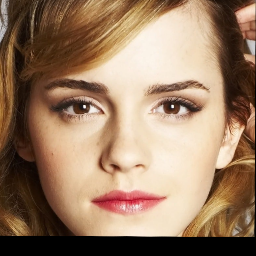} & \includegraphics[width=0.115\textwidth]{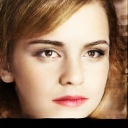} & \includegraphics[width=0.115\textwidth]{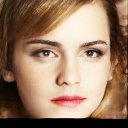} & \includegraphics[width=0.115\textwidth]{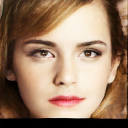} & \includegraphics[width=0.115\textwidth]{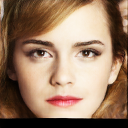} & \includegraphics[width=0.115\textwidth]{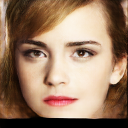} & \includegraphics[width=0.115\textwidth]{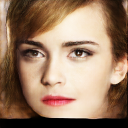} & \includegraphics[width=0.115\textwidth]{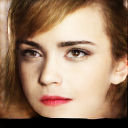} & \includegraphics[width=0.115\textwidth]{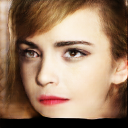} \\
    \rotatebox{90}{\hspace{0.5cm} Ours} &
    \includegraphics[width=0.115\textwidth]{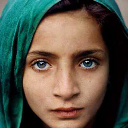} & \includegraphics[width=0.115\textwidth]{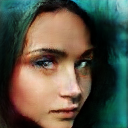} & \includegraphics[width=0.115\textwidth]{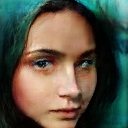} & \includegraphics[width=0.115\textwidth]{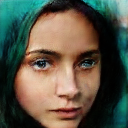} & \includegraphics[width=0.115\textwidth]{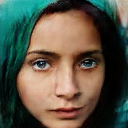} & \includegraphics[width=0.115\textwidth]{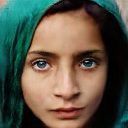} & \includegraphics[width=0.115\textwidth]{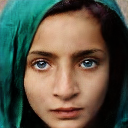} & \includegraphics[width=0.115\textwidth]{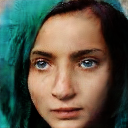} & \includegraphics[width=0.115\textwidth]{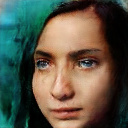} \\
    \rotatebox{90}{\hspace{0.2cm} ConfigNet} &
    \includegraphics[width=0.115\textwidth]{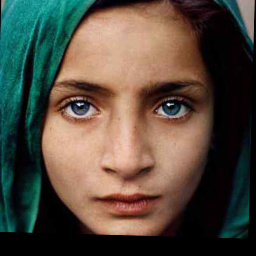} & \includegraphics[width=0.115\textwidth]{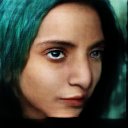} & \includegraphics[width=0.115\textwidth]{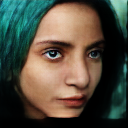} & \includegraphics[width=0.115\textwidth]{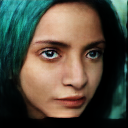} & \includegraphics[width=0.115\textwidth]{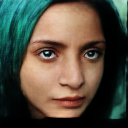} & \includegraphics[width=0.115\textwidth]{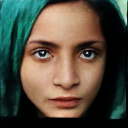} & \includegraphics[width=0.115\textwidth]{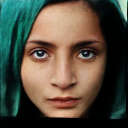} & \includegraphics[width=0.115\textwidth]{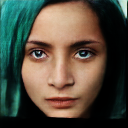} & \includegraphics[width=0.115\textwidth]{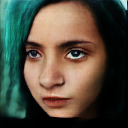} \\
	\end{tabular}}
	\caption{Qualitative comparison against ConfigNet \cite{kowalskiECCV2020} on downloaded web images. For each input image, the top row is our method, while the bottom row is ConfigNet.}
	\label{fig:comparison_cfgnet}
\end{figure*}
